# Supplementary material for: Learning Label Hierarchy with Supervised Contrastive Learning
Source: arXiv:2402.00232 source file (2024-01-31)
Supplement: Supplementary file 1 [file hie_appendix.tex]

\begin{figure}[!tbp]
  \centering
    \includegraphics[width=0.5\textwidth]{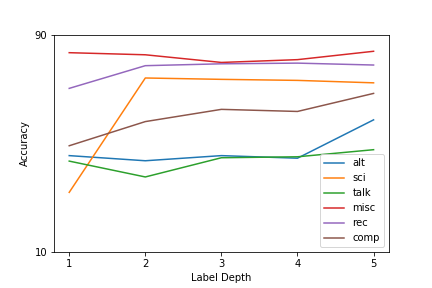}
  \caption{The highest level parent node performance with different label hierarchies.}
  \label{fig:hie2}
\end{figure}
